# Supplementary material for: Analytical Derivation of Outage Correlation in Random Media Access with Application to Average Consensus in Wireless Networks: Extended Paper Version
Source: arXiv:2007.09120 source file (2020-07-17)
Supplement: Supplementary file 1 [file 999_appendix_alt.tex]

\appendix
Here we do the ugly stuff!!
\subsection{Proof of XYZ}

\newpage

\textbf{alter Kram} 

\begin{prp}
\comment{Rephrasing full Prop. just for convenience while writing the paper}
%\label{prp:slotCorrelations}

\begin{abc}
\item \comment{verify!!} Let $i \ne j$ and $k \ne l.$ Then
		%$ $\E X_{ij}X_{il} = \frac{1}{m^{n-1}} \sum_{\substack{c_{\iota = 0}\\ \iota \ne i}}^{1}\phi $ $
	$$\begin{aligned}\label{eqn:removed}\E[&X_{ij}X_{kl} \vert S_i = S_k] \\&= \frac{1}{m^{n-1}} \sum_{c_1, \dots, c_{i-1},c_{i+1},\dots c_n = 0}^{1}\left[ \vphantom{\frac{x}{y}}\phi(c)\right.\\
			& \ds\ds \cdot \Pr(\frac{P_{ij}}{N+ \sum_{\nu \ne i,j}^{}c_\nu P_{\nu j}}\ge \theta)\\ 
		&\left.\ds\ds \cdot \Pr(\frac{P_{kl}}{N+ \sum_{\nu \ne k,l}^{}c_\nu P_{\nu l}}\ge \theta)\right],
		\end{aligned}$$
		where $\phi(c) := \prod_{\nu \ne i}(m-1)^{1-c_\nu}.$

In Particular, $\E X_{ij}X_{il} = \E [X_{ij}X_{il} \vert S_i = S_i]$ can be expressed by ().
%	\item Let $i \ne j$ and $i \ne l.$ Then
%		%$$\E X_{ij}X_{il} = \frac{1}{m^{n-1}} \sum_{\substack{c_{\iota = 0}\\ \iota \ne i}}^{1}\phi $$
%		$$\begin{aligned}\E X_{ij}&X_{il} \\&= \frac{1}{m^{n-1}} \sum_{c_1, \dots, c_{i-1},c_{i+1},\dots c_n = 0}^{1}\left[ \vphantom{\frac{x}{y}}\phi(c)\right.\\
%			& \ds\ds \cdot \Pr(\frac{P_{ij}}{N+ \sum_{\nu \ne i,j}^{}c_\nu P_{\nu j}}\ge \theta)\\ 
%		&\left.\ds\ds \cdot \Pr(\frac{P_{il}}{N+ \sum_{\nu \ne i,l}^{}c_\nu P_{\nu l}}\ge \theta)\right],
%		\end{aligned}$$
%		where $\phi(c) := \prod_{\nu \ne i}(m-1)^{1-c_\nu}.$
%
%		Note that $\sum_{}^{}\phi = m^{n-1}.$

	\item Let $k\ne i, l \ne j, i\ne l, k\ne j.$ Then
		$$ \begin{aligned}&\E X_{ij}X_{kl} \ds \ds \\
			&= \frac{m-1}{m^{n-1}}  \csum{2} \left[ \vphantom{\frac{x}{y}}\psi_m(c)\right.\\
			&\ds\ds\ds\ds \cdot \Pr\left(\frac{P_{ij}}{N+ \sum_{\nu \ne i,j,k}^{}\delta_{c_\nu, 1}P_{\nu,j}} \ge \theta  \right) \\ 
		&\left.\ds\ds\ds\ds  \cdot \Pr\left(\frac{P_{kl}}{N+ \sum_{\nu \ne k,l,i}^{}\delta_{c_\nu, 2}P_{ \nu,l }} \ge \theta   \right)\right]\\
			&\ds\ds  + \frac{1}{m^{n-1}}\csum{1}\left[ \vphantom{\frac{x}{y}}\phi_m(c)\right.\\
			&\ds\ds \ds\ds\cdot \Pr\left(\frac{P_{ij}}{N+\sum_{\nu \ne i,j,k}^{}c_\nu P_{\nu j}+ P_{kj}} \ge \theta\right)\\
		&\left.\ds\ds\ds\ds  \cdot \Pr\left( \frac{P_{kl}}{N + \sum_{\nu \ne k,l,i}^{}c_\nu P_{\nu l} + P_{il}} \ge \theta \right)\right]
			,\end{aligned}$$
		where we use the following notational abbreviations, for $d= 1,2$:
		%$$\csum{2} (\dots) := \prod_{\substack{\iota = 1\\ \iota\ne i,k }}^n \sum_{c_\iota=0}^{2}\left( \dots \right),$$
		$$\csum{d} (\dots) := \prod_{\substack{\nu = 1\\ \nu\ne i,k }}^n \sum_{c_\nu=0}^{d}\left( \dots \right),$$
		and within the sums' scope:
		$$\psi_m(c) := \prod_{\substack{\nu = 1\\ \nu \ne i,k}}^n (m-2)^{1-\delta_{c_\nu, 1}}.$$
		and
		$$\phi_m(c) :=  ??$$

		%where, for any function $f:\R^n \sra \R,$
		%$$\csum{2} f(c_1, \dots, c_n) := \prod_{\substack{\iota = 1\\ \iota\ne i,k }}^n \sum_{c_\iota=0}^{2}f(c_1, \dots, c_n)$$
		%(note that we have not excluded $c_i$ and $c_k$ in the argument list of $f$ for the sake of notational convenience).
		
	\end{abc}
\end{prp} 
\begin{proof}
If $j=l$, we have 
%$$\begin{aligned}\E &[X_{ij}X_{kj}\vert S_i = S_k] \\ &=\Pr\left( \frac{P_{ij}}{N + \sum_{\nu \ne i,j,k}^{}\delta_{S_i S_\nu}P_{\nu j} + P_{kj}}\ge \theta\right. \\ &\left.\ds\ds\ds\ds \mbox{ and } \frac{P_{kj}}{N+\sum_{\nu\ne i,j,k}^{}\delta_{S_i S_{\nu}}P_{\nu j} + P_{ij}}\ge \theta \right)
$$\begin{aligned}\E &[X_{ij}X_{kj}\vert S_i = S_k] \\ &=\Pr\left( \frac{P_{ij}}{N + J_{ijk} + P_{kj}}\ge \theta \mbox{ and } \frac{P_{kj}}{N+ J_{ijk} + P_{ij}}\ge \theta \right)
\end{aligned}$$
where $J_{ijk} = \sum_{\nu \ne i,j,k}^{}\delta_{S_i S_\nu}P_{\nu j}.$ However, since $\theta \ge 1,$ and $N > 0$ only one event can occur at the same time (otherwise: $P_{kl}(1-\theta^2) \ge (N+J_{ijk})(1+\theta)$ a contradiction.
\end{proof}

\subsection{Proof of XYZ}
blaa\\[2cm]

\subsection{Aussortiert}
\textbf{ Aussortiert:} \\

\begin{prp}
\begin{abc}
\item \comment{verify!!} Let $i \ne j, k \ne l,$ and $(i,j) \ne (k,l).$ Then
		%$ $\E X_{ij}X_{il} = \frac{1}{m^{n-1}} \sum_{\substack{c_{\iota = 0}\\ \iota \ne i}}^{1}\phi $ $
	\begin{equation}\begin{aligned}\label{eqn:removed2}\E[&X_{ij}X_{kl} \vert S_i = S_k] \\&= \frac{1-\delta_{lj}}{m^{n-1}} \sum_{\substack{c_1, \dots, c_{i-1},\\c_{i+1},\dots c_n = 0}}^{1}\phi(c)\cdot \alpha_{ij}(c)\cdot \alpha_{kl}(c) \end{aligned}\end{equation}
	where $c = (c_1, \dots, c_{i-1}, c_{i+1}, \dots, c_n) \in \left\{ 0,1 \right\}^{n-1},$
		$$\begin{aligned}\phi(c) &:= \prod_{\nu \ne i}(m-1)^{1-c_\nu},\\
			\alpha_{i'j'}(c) &: = \Pr\left(\frac{P_{i'j'}}{N+\sum_{\nu\ne i',j'}^{}c_\nu P_{\nu j'}} \ge \theta\right),\\
		\end{aligned}$$
		for $i' \ne j', \; d = 1,2.$

In particular, $\E X_{ij}X_{il} = \E [X_{ij}X_{il} \vert S_i = S_i]$ can be expressed by (\ref{eqn:formulaSameSlot}). 	
 	\item Let $k\ne i, l \ne j, i\ne l, k\ne j.$ Then
		%$$ \begin{aligned}&\E X_{ij}X_{kl} \ds \ds \\
		$$ \begin{aligned}\E X_{ij}X_{kl} = \frac{m-1}{m^{n-1}}  &\csum{2} \psi(c)\cdot \beta_{ijk}^{(1)}(c) \cdot \beta_{kli}^{(2)}(c)\\
			 + \frac{1}{m^{n-1}}&\csum{1}\varphi(c) \cdot  \gamma_{ijk}(c) \cdot \gamma_{kli}(c)
			,\end{aligned}$$
		where we use the following notational abbreviations, for $d= 1,2$:
		%$$\csum{2} (\dots) := \prod_{\substack{\iota = 1\\ \iota\ne i,k }}^n \sum_{c_\iota=0}^{2}\left( \dots \right),$$
		$$\csum{d} (\dots) := \prod_{\substack{\nu = 1\\ \nu\ne i,k }}^n \sum_{c_\nu=0}^{d}\left( \dots \right),$$
		%and within the sums' scope:
		and for $c = (c_1, \dots, c_{\mu-1},c_{\mu+1}, c_{M-1}, c_{M+1}) \in \left\{ 0,1,2 \right\}^{n-2}, \ds \mu = \mbox{min}(i,k), M = \mbox{max}(i,k)$

		$$\begin{aligned} \psi(c) &:= \prod_{\substack{\nu = 1\\ \nu \ne i,k}}^n (m-2)^{1-\delta_{c_\nu, 1}}.\\
				  \varphi(c) &:=  ??\\
				  \beta_{i'j'k'}^{(d)}(c) &: = \Pr\left(\frac{P_{i'j'}}{N+\sum_{\nu\ne i',j',k'}^{}\delta_{c_\nu d} P_{\nu j'}} \ge \theta  \right),\\
				  \gamma_{i'j'k'}(c) &: = \Pr\left(\frac{P_{i'j'}}{N+\sum_{\nu\ne i',j',k'}^{}c_\nu P_{\nu j'} + P_{k'j'}} \ge \theta\right),\\
		\end{aligned}$$

		%where, for any function $f:\R^n \sra \R,$
		%$$\csum{2} f(c_1, \dots, c_n) := \prod_{\substack{\iota = 1\\ \iota\ne i,k }}^n \sum_{c_\iota=0}^{2}f(c_1, \dots, c_n)$$
		%(note that we have not excluded $c_i$ and $c_k$ in the argument list of $f$ for the sake of notational convenience). 

\end{abc}
	
\end{prp}<++>

\begin{prp}
%\label{prp:slotCorrelations}
Let $\theta \ge 1.$
\begin{abc}
\item Let $i \ne j, k \ne l,$ and $(i,j) \ne (k,l).$ Then
		%$ $\E X_{ij}X_{il} = \frac{1}{m^{n-1}} \sum_{\substack{c_{\iota = 0}\\ \iota \ne i}}^{1}\phi $ $
                                        %\label{eqn:formulaSameSlot}
	\begin{equation}\begin{aligned}\E[&X_{ij}X_{kl} \vert S_i = S_k] \\&= \frac{1-\delta_{lj}}{m^{n-2}} \prod_{\substack{\nu = 1\\ \nu\ne i,k }}^n \sum_{c_\nu=0}^{1}\phi(c)\cdot \alpha_{ij}(c)\cdot \alpha_{kl}(c) \end{aligned}\end{equation}
where\footnote{the product with subsequent sum in (\ref{eqn:formulaSameSlot}) is meant to expand into an $n-2$-fold sum over $c_\nu,\ \nu \ne i,k.$}
%\label{eqn:alpha_phi} 
\begin{subequations}\begin{align}\phi(c) &:= \prod_{\nu \ne i,k}(m-1)^{1-c_\nu},\\
			%\alpha_{i'j'}(c) &: = \Pr\left(\frac{P_{i'j'}}{N+\sum_{\nu\ne i',j'}^{}c_\nu P_{\nu j'}} \ge \theta\right),\\
			%\alpha_{xy}(c) &: = \Pr\left(\frac{P_{xy}}{N+\sum_{\nu\ne x,y}^{}c_\nu P_{\nu y}} \ge \theta\right),
			\alpha_{xyz}(c) &: = \Pr\left(\frac{P_{xy}}{N+\sum_{\nu\ne x,y,z}^{}c_\nu P_{\nu y} + P_{zy}} \ge \theta\right),
		\end{align}\end{subequations}
and where $c = (c_\nu) \in   \left\{ 0,1 \right\}^{n-2},$
	$$c = (c_1, \dots, c_{\mu-1},c_{\mu+1},\dots, c_{M-1}, c_{M+1},\dots, c_n),$$
$\mu = \mbox{min}(i,k), M = \mbox{max}(i,k).$

In particular, $\E X_{ij}X_{il} = \E [X_{ij}X_{il} \vert S_i = S_i]$ can be expressed by (\ref{eqn:formulaSameSlot}).

%	\item Let $i \ne j$ and $i \ne l.$ Then
%		%$$\E X_{ij}X_{il} = \frac{1}{m^{n-1}} \sum_{\substack{c_{\iota = 0}\\ \iota \ne i}}^{1}\phi $$
%		$$\begin{aligned}\E X_{ij}&X_{il} \\&= \frac{1}{m^{n-1}} \sum_{c_1, \dots, c_{i-1},c_{i+1},\dots c_n = 0}^{1}\left[ \vphantom{\frac{x}{y}}\phi(c)\right.\\
%			& \ds\ds \cdot \Pr(\frac{P_{ij}}{N+ \sum_{\nu \ne i,j}^{}c_\nu P_{\nu j}}\ge \theta)\\ 
%		&\left.\ds\ds \cdot \Pr(\frac{P_{il}}{N+ \sum_{\nu \ne i,l}^{}c_\nu P_{\nu l}}\ge \theta)\right],
%		\end{aligned}$$
%		where $\phi(c) := \prod_{\nu \ne i}(m-1)^{1-c_\nu}.$
%
%		Note that $\sum_{}^{}\phi = m^{n-1}.$

\item Let $i \ne j, k \ne l,$ and $i \ne k.$ Then
	\begin{equation*} \begin{aligned} &\E \left[ X_{ij}X_{kl}\vert S_i \ne S_k \right] = \left( \E X_{ij} \right)\left( \E X_{kl} \right)\\
			%= &\left( \E X_{ij} \right)\left( \E X_{kl} \right)\\
			& \ds\ds - \frac{1}{m^{n-1}-1} \prod_{\substack{\nu = 1\\\nu \ne i,k}}^n \sum_{c_\nu = 0}^{1}(\phi(c)\cdot \beta_{ijk}(c)\cdot \beta_{kli})(c) 
		\end{aligned}\end{equation*}
	
	where $\phi(c)$ is defined in (\ref{eqn:alpha_phi}) and $c = (c_\nu)$ as in the first part.

		%$$\begin{aligned} \psi(c) &:=  ??\\
				  %\beta_{xyz}(c) &: = \Pr\left(\frac{P_{xy}}{N+\sum_{\nu\ne x,y,z}^{}c_\nu P_{\nu y} + P_{zy}} \ge \theta\right),\\ \end{aligned}$$ 
	$$\beta_{xyz}(c) : = \Pr\left(\frac{P_{xy}}{N+\sum_{\nu\ne x,y,z}^{}c_\nu P_{\nu y} + P_{zy}} \ge \theta\right),$$

	\end{abc}
\end{prp}

\textbf{ Leider ein bloeder Fehler unterlaufen. Alles falsch } 
\begin{prp}
%\label{prp:slotCorrelations}
Let $\theta \ge 1,$ let $N > 0$, let $i \ne j, k \ne l,$ and $(i,j) \ne (k,l),$ and define
%\label{eqn:formulaSameSlot}
\begin{equation}\begin{aligned}\Gamma_{ijkl}  :=  \prod_{\substack{\nu = 1\\ \nu\ne i,k }}^n \sum_{c_\nu=0}^{1}\phi(c)\cdot \alpha_{ijk}(c)\cdot \alpha_{kli}(c) \end{aligned}\end{equation}
where\footnote{the product with subsequent sum in (\ref{eqn:formulaSameSlot}) is meant to expand into an $n-2$-fold sum over $c_\nu,\ \nu \ne i,k.$}
% \label{eqn:alpha_phi}
\begin{subequations}\begin{align} \phi(c) &:= \prod_{\nu \ne i,k}(m-1)^{1-c_\nu},\\
			%\alpha_{i'j'}(c) &: = \Pr\left(\frac{P_{i'j'}}{N+\sum_{\nu\ne i',j'}^{}c_\nu P_{\nu j'}} \ge \theta\right),\\
			%\alpha_{xy}(c) &: = \Pr\left(\frac{P_{xy}}{N+\sum_{\nu\ne x,y}^{}c_\nu P_{\nu y}} \ge \theta\right),
		\alpha_{xyz}(c) &: = \Pr\left(\frac{P_{xy}}{N+\sum_{\nu\ne x,y,z}^{}c_\nu P_{\nu y} + (1-\delta_{xz})P_{zy}} \ge \theta\right),
		\end{align}\end{subequations}
and where $c = (c_\nu) \in   \left\{ 0,1 \right\}^{n-2+\delta_{ik}},$
	$$c = (c_1, \dots, c_{\mu-1},c_{\mu+1},\dots, c_{M-1}, c_{M+1},\dots, c_n),$$
$\mu = \mbox{min}(i,k), M = \mbox{max}(i,k).$  

\begin{abc}\item Then we have 
		$$\E[X_{ij}X_{kl} \vert S_i = S_k] = \frac{1-\delta_{lj}}{m^{n-2+\delta_{ik}}} \cdot \Gamma_{ijkl}.$$
		In particular, $\E X_{ij}X_{il} = \E [X_{ij}X_{il} \vert S_i = S_i]$ can be expressed in virtue of (\ref{eqn:formulaSameSlot}) which gives for $j \ne l$
		$$\cov(X_{ij}, X_{il}) = \frac{ \Gamma_{ijil}}{m^{n-2+\delta_{ik}}}  - \E X_{ij} \E X_{kl}.$$

\item If $i \ne k,$ then
	%\begin{equation*} \begin{aligned} &\E \left[ X_{ij}X_{kl}\vert S_i \ne S_k \right] = \left( \E X_{ij} \right)\left( \E X_{kl} \right)\\
			%& \ds\ds - \frac{1}{m^{n-1}-1} \prod_{\substack{\nu = 1\\\nu \ne i,k}}^n \sum_{c_\nu = 0}^{1}(\phi(c)\cdot \beta_{ijk}(c)\cdot \beta_{kli})(c) 
		%\end{aligned}\end{equation*}

	\begin{equation*} \begin{aligned} \E \left[ X_{ij}X_{kl}\vert S_i \ne S_k \right] &= \frac{m \cdot \E X_{ij} \E X_{kl} - \Gamma_{ijkl}/{m^{n-1}}}{m-1}\\
			%& \ds\ds - \frac{1}{m^{n-1}(m-1)} \cdot \Gamma_{ijkl},
		\end{aligned}\end{equation*} 	
	%\begin{equation*} \begin{aligned} \E \left[ X_{ij}X_{kl}\vert S_i \ne S_k \right] &= \frac{m}{m-1}  \E X_{ij} \E X_{kl} \\
			%& \ds\ds - \frac{1}{m^{n-1}(m-1)} \cdot \Gamma_{ijkl},
		%\end{aligned}\end{equation*} 	

		%$$\begin{aligned} \psi(c) &:=  ??\\
				  %\beta_{xyz}(c) &: = \Pr\left(\frac{P_{xy}}{N+\sum_{\nu\ne x,y,z}^{}c_\nu P_{\nu y} + P_{zy}} \ge \theta\right),\\ \end{aligned}$$ 
	%$$\beta_{xyz}(c) : = \Pr\left(\frac{P_{xy}}{N+\sum_{\nu\ne x,y,z}^{}c_\nu P_{\nu y} + P_{zy}} \ge \theta\right),$$
		
hence
	$$\cov(X_{ij}, X_{kl}) = \frac{\Gamma_{ijkl} }{m^{n-1}} \cdot (1- \delta_{il} - \frac{1}{m}).$$
	\end{abc}
\end{prp}

 	There are two further aspects we have to consider: Sending nodes cannot receive (singular antenna case) and multiple receptions at some node at the same time (i.e. in the same slot) are impossible (\comment{improvement?}). We will only model the former aspect in our formal treatment. However, we keep track of the latter case in simulations and show (\comment{verify!!}) that this happens rarely such that our analysis is still meaningful. \comment{Maybe also add estimates somewhere}. In this sense we define successful packet reception $Y_{ij}, \, 1 \le i, j \le n,\; i \ne j,$ as Bernoulli variables having the following properties: \comment{kann man das verbessern durch eine richtige Defintion, die 100\%ig konsistent ist? }
	$$\begin{aligned}\E Y_{ij} &= \E[ (1-\delta_{S_iS_j}) \cdot X_{ij}]\\
		\E Y_{ij}Y_{kl} &= \E[ (1-\delta_{il}\delta_{S_iS_k}) (1-\delta_{jk}\delta_{S_iS_k})\cdot X_{ij}X_{kl} ],\end{aligned}$$
for $i \ne k.$ \comment{fehlt da noch was?}

The following Lemma follows readily:
\begin{lem} 
	(a) For $i =k$ we have 
		$$\E Y_{ij}Y_{kl} = \E X_{ij}X_{il}.$$

	(b) We have for $i \ne k:$
	$$\begin{aligned}\E Y_{ij} &= (1-\frac{1}{m}) \cdot \E X_{ij}\\
		%\E Y_{ij}Y_{kl} &= (1-\frac{1}{m}) \cdot \E X_{ij}X_{kl} + \frac{1}{m} \E\left[ X_{ij} X_{kl}  \vert S_i = S_k \right].\end{aligned}$ $ 
		\E Y_{ij}Y_{kl} &= \E X_{ij}X_{kl} - \frac{\delta_{il}+\delta_{jk} - \delta_{il}\delta_{jk}}{m} \E\left[ X_{ij} X_{kl}  \vert S_i = S_k \right].\end{aligned}$$
\end{lem}
\begin{proof}
Part (a) is clear. See Appendix.	
\end{proof}
